# Supplementary material for: Understanding the Interplay of Scale, Data, and Bias in Language Models: A Case Study with BERT
Source: arXiv:2407.21058 source file (2024-07-25)
Supplement: Supplementary file 1 [file appendix.tex]

\appendix
\section{Appendices}
\label{sec:appendix}

%\section{Supplemental Material}
%\label{sec:supplemental}
%\section{Impact of Pre-Training Data}

%\paragraph{Toxicity:}
%In Figure %~\ref{fig:upstream_sentiment_timeline}  we plot the average negative sentiment over identities for intermediate checkpoints of models during their pre-training on Wikipedia and CC-100.
%from mid-point checkpoints for the different scales of BERT trained on a single dataset.
%We observe that models pre-trained on CC-100, in general, result in higher negative sentiment associations over identity groups over the course of the pre-training period.
% TODO:Ali: isn't this result same as Figure 1 a)?

\section{Social Impact Statement} 
Our work contributes to ongoing scientific discourse about the risks of large language models. We first provide empirical measurements of biased language, and study its relation to model size and training data used. These results highlight the crucial role of training data in the adverse outcomes of LLMs. We hope this encourages future work to more deeply investigate the role of data when studying scaling laws
